# Supplementary material for: Anisotropic electron gas in a hyperbolic van der Waals material
Source: arXiv:2602.01072 source file (2026-02-14)

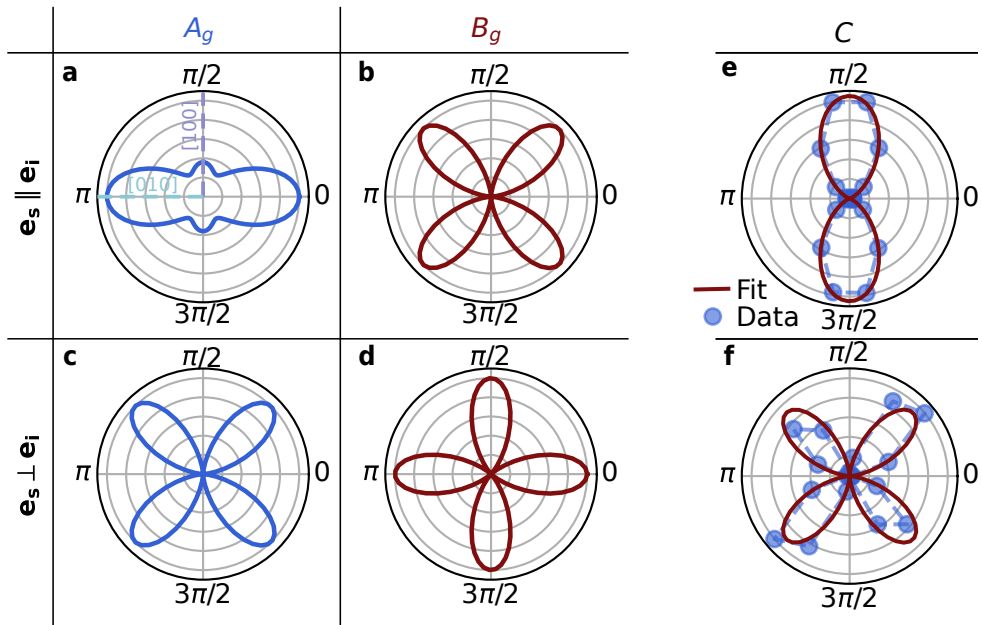

Supplement: Supplementary file 1 [file SI_ARPR_Theory.pdf]
